# Supplementary material for: Im2Vec: Synthesizing Vector Graphics without Vector Supervision
Source: arXiv:2102.02798 source file (2021-04-01)
Supplement: Supplementary file 1 [file 07_Supplementary.tex]

\section{More Qualitative Results}
A sampling of 1000 random samples from the latent space of \Fonts dataset is included in the supplemental folder to demonstrate the diversity of the results generated by \name. We also include 256x256 raster images of the vector graphics shapes. We post process the raster images to remove curves that rasterize to less than $10\times10$ pixels. 

\section{Network Architecture}
Our Encoder network contains 5 2D convolution residual  blocks, with [32, 64, 128, 256, 512] filters respectively. All the convolution layers have kernel size 3, stride 2 and zero pad the input by 1 pixel in both spatial dimensions. 
The convolutional layers are followed by two parallel fully-connecter layers that each output a vector of size 128; they represent the mean and variance for the latent embedding. 
Our Path decoder has 6 1D convolution layers with [170, 340, 340, 340, 340, 340, 2] channels. All the 1D convolutions have kernel size 3, stride 1 and circular padding of the input by 1 tap.
Our auxiliary network contains 4 fully-connected layers with [256, 256, 256, 3] channels, respectively.
The sample deformation network contains 3 1D convolution layers with [340, 340, 1] channels, all the convolution layers have the same kernel size, stride and padding as the 1D convolution layers in path decoder.
All layers are followed by ReLU activations, except the last layer of the path decoder which is followed by a sigmoid activation.

\section{Chamfer Distance}
An alternative, commonly used metric to measure the reconstruction accuracy for geometric objects is the Chamfer distance.
For two point sets X, Y, the Chamfer distance is defined as:
\begin{equation}
\sum_{x \in X} \operatorname{min}_{y \in Y} \|x- y\|^2 + \sum_{y \in Y} \operatorname{min}_{x \in X} \|x- y\|^2.
\end{equation}
In Table~\ref{tab:chamfer_comparison}, we show the bidirectional Chamfer distance computed between the synthesized and ground truth geometries, with points sampled uniformly along the shape boundaries (according to the path parameterization).
Unlike the pixel-space metrics we report in the main paper, this evaluation suggests our model underperforms the baselines. This is misleading.
%
% The table shows that \name does not perform well compared to the baselines when measuring reconstruction loss using the Chamfer distance.
%
% Whereas comparisons from the main paper show that \name outperforms the baselines in reconstruction loss when measured in pixel space.
%
%This is due to the non-linear relationship between vector graphics parameters and image space appearance. As multiple vector graphics parameterization can raster to exactly the same image.
%
As shown by Smirnov~\etal~\cite{smirnov2020deep}, the Chamfer distance varies wildly, depending on the sampling pattern (and the parameterization, by extension). This adversely impacts our method.
The baselines (DeepSVG and SVG-VAE) are optimized to regress the ground truth vector parameterization, which leads to a lower Chamfer loss, despite worse perceptual fidelity.
Conversely, our method is trained on raster data only. It does not seek to retrieve the ground truth parameterization of the curve, but rather to faithfully capture the (rasterized) appearance. Therefore, our model achieves higher fidelity, despite a higher Chamfer distance.
%Therefore  we argue that bidirectional chamfer distance is not the right metric for perceptual evaluation of solid object reconstruction performance.
%
\begin{table}
  \centering
  \caption{\label{tab:chamfer_comparison}
    {\bf Reconstruction quality.} Comparison of Bidirectional Chamfer Distance reconstruction losses for various methods
    and datasets.
}
  \begin{tabular}{r c}
    \toprule
  & \Fonts  \\ 
  \midrule
    ImageVAE & \ding{53} \\
    SVG-VAE & 0.168 \\
    DeepSVG & 0.136 \\
    \name (Ours) & 0.279  \\
    \bottomrule
  \end{tabular}
\end{table}

\begin{figure}
    \centering
    \begin{subfigure}[t!]{\linewidth}
        \centering
        \includegraphics[width=\linewidth]{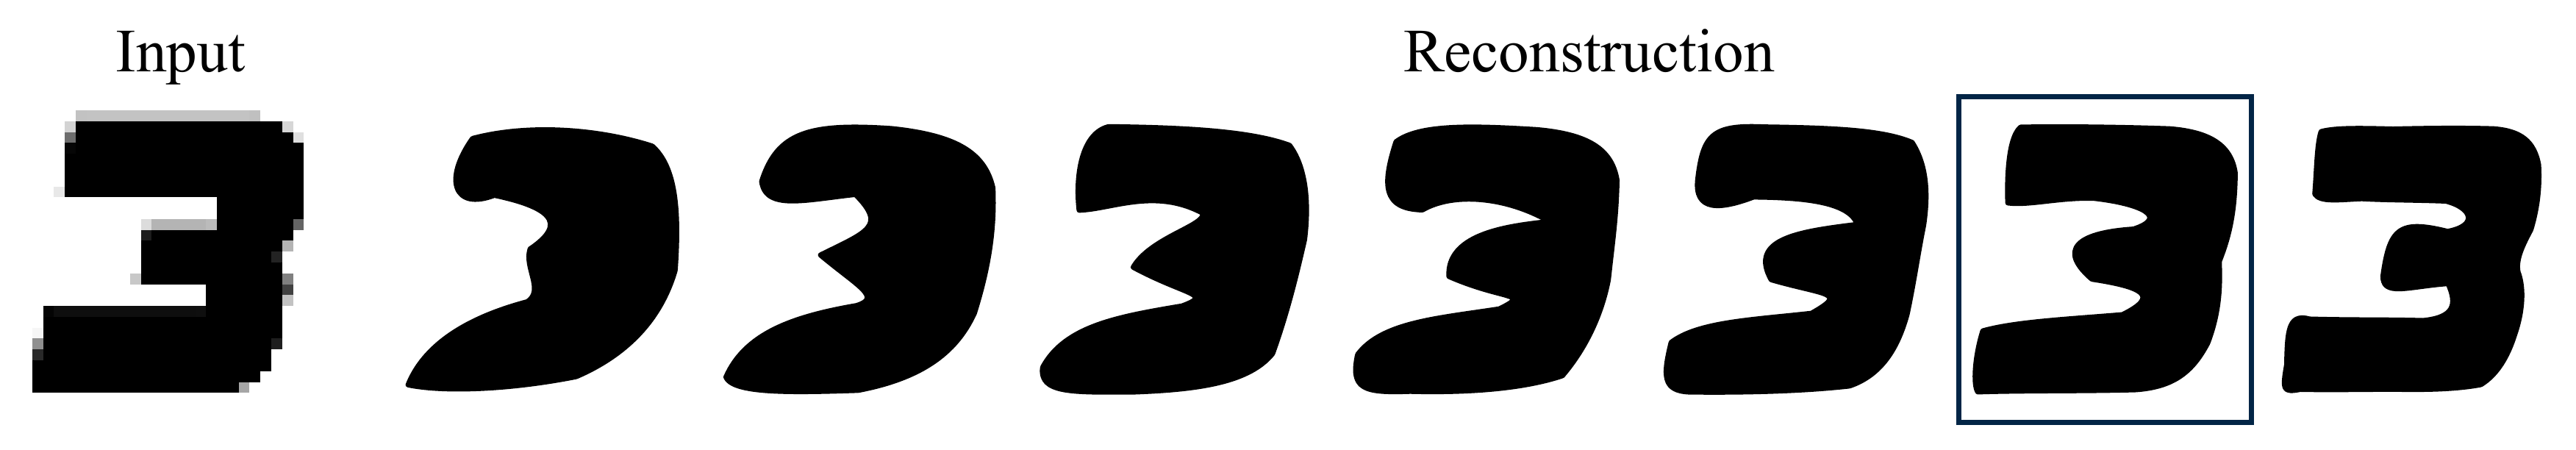}
        \caption{\label{fig:error_vs_segments_supp}visual fidelity vs.\ number of
        segments}
    \end{subfigure}
    \begin{subfigure}[b]{\linewidth}
        \centering
        \includegraphics[width=0.8\linewidth]{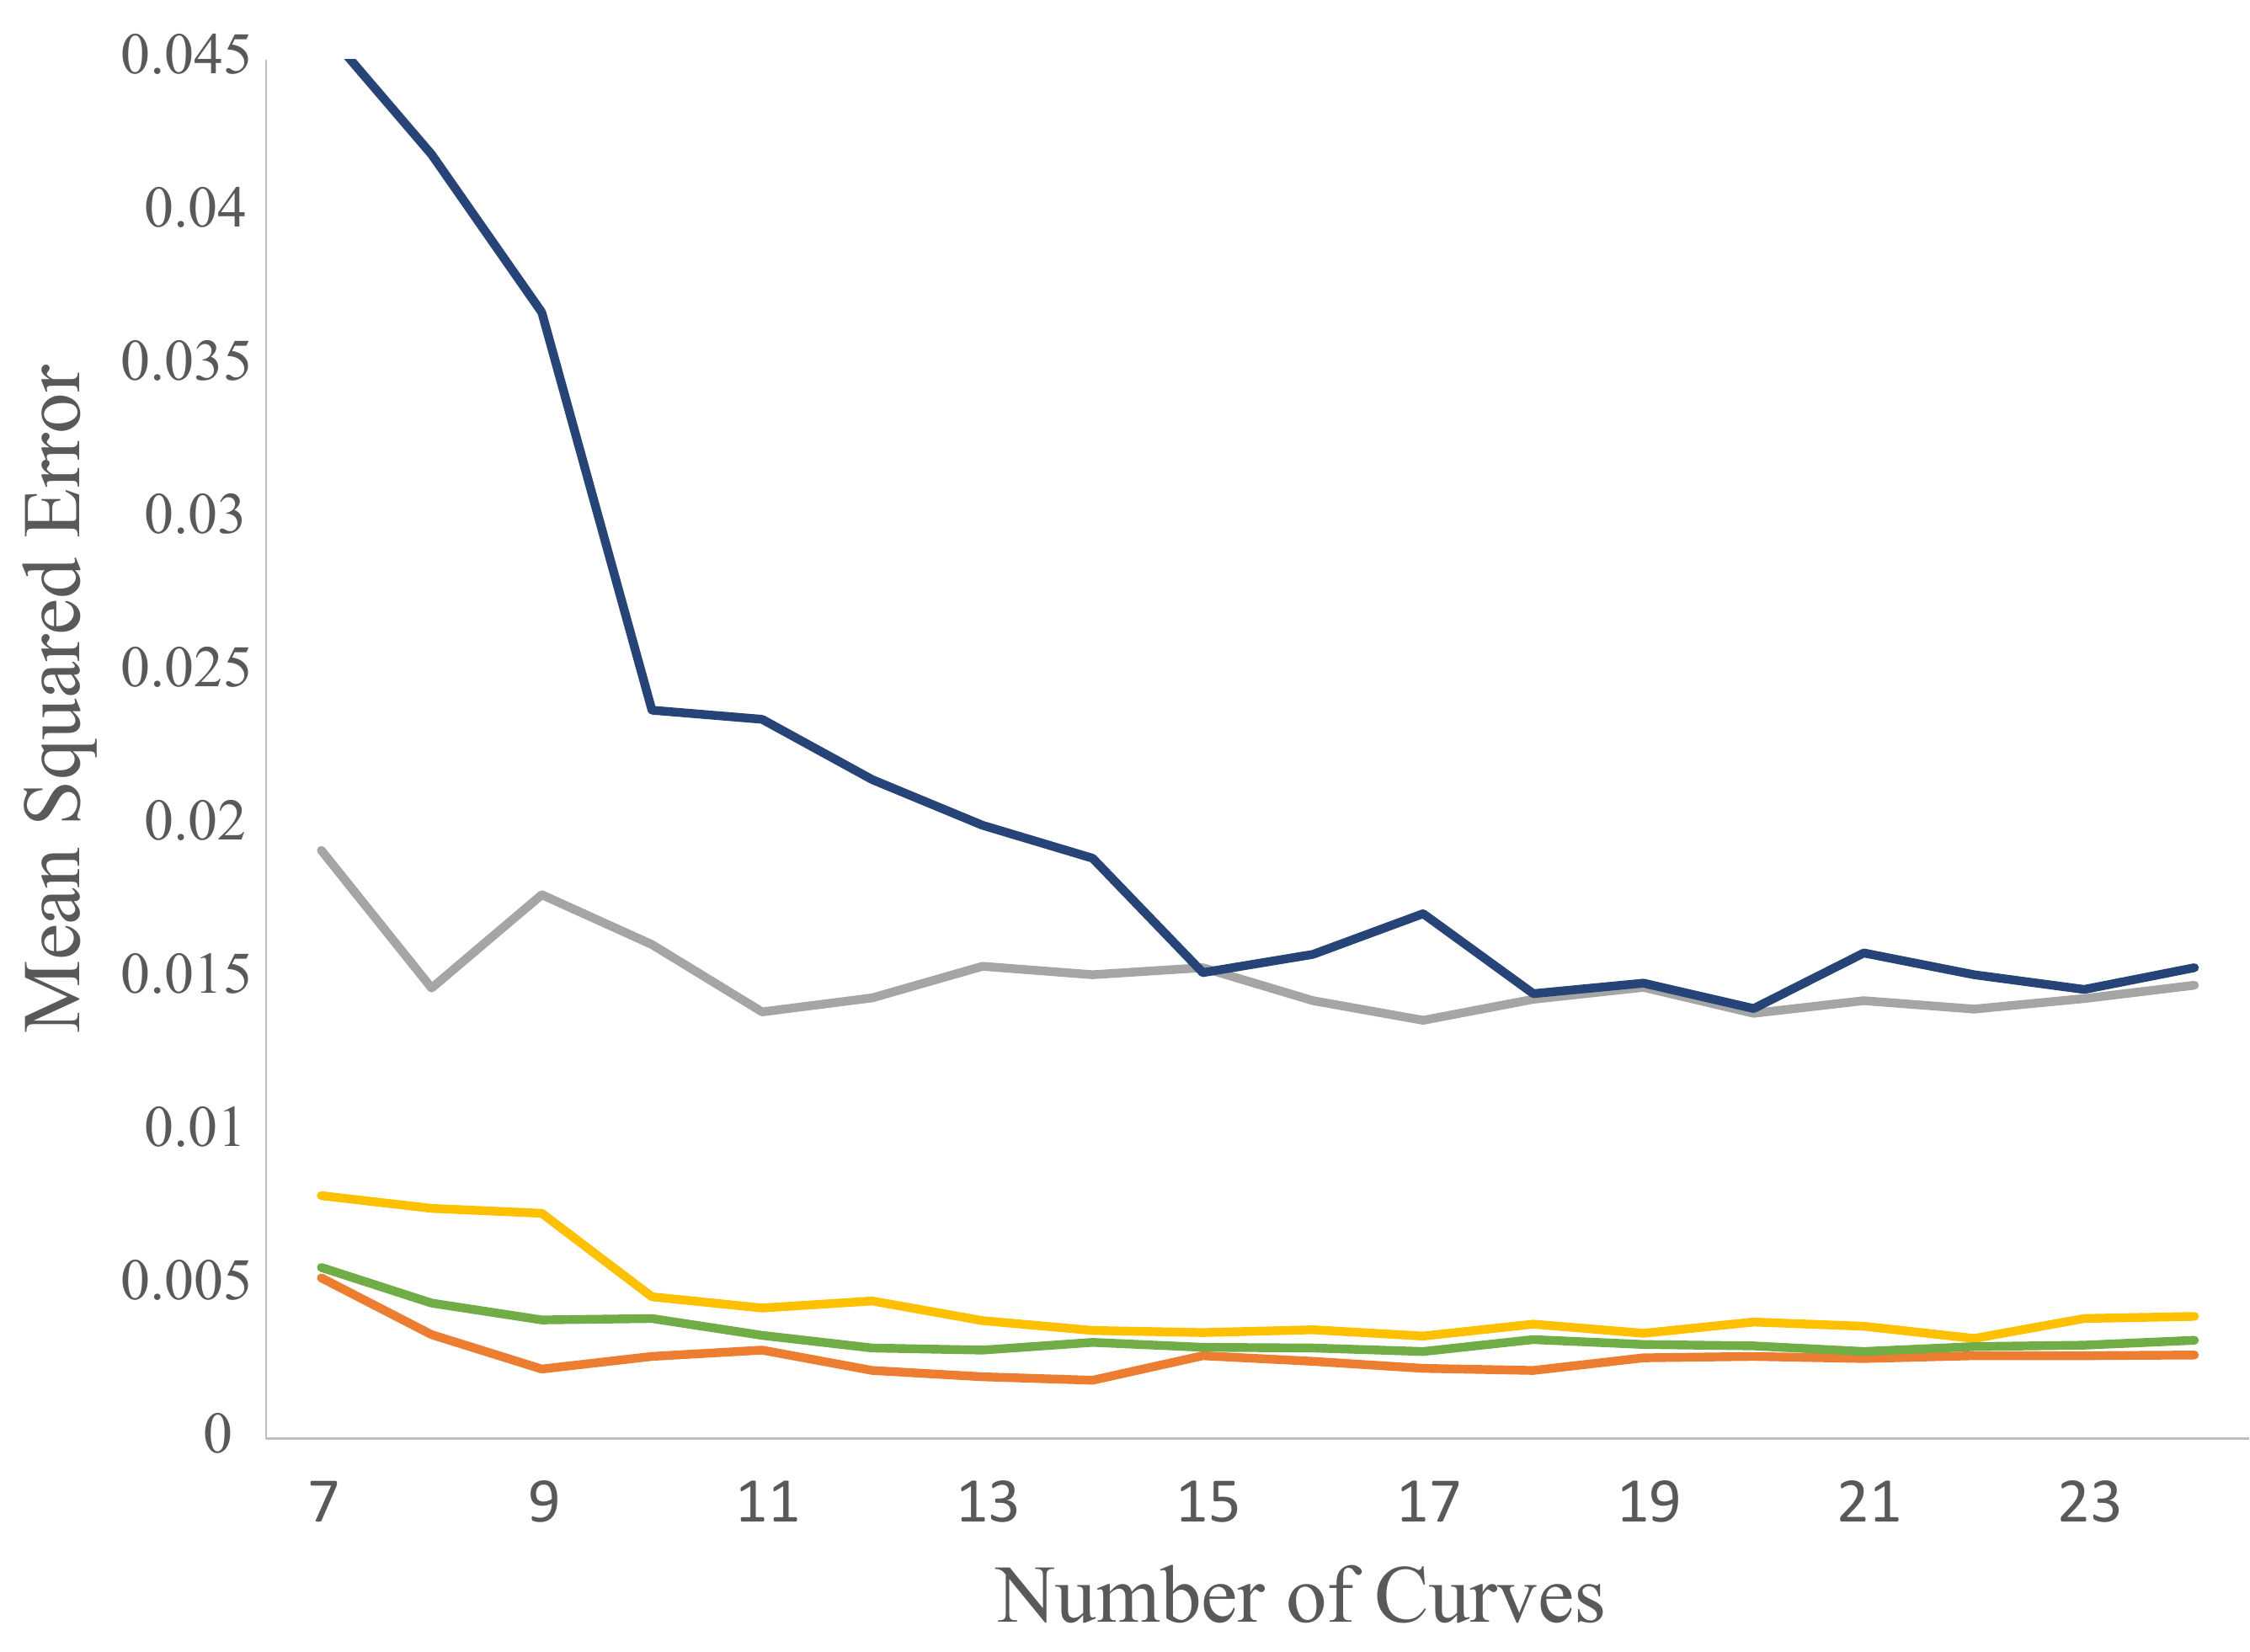}
        \caption{error vs.\ number of segments; ground truth\label{fig:graph_gt}}
    \end{subfigure}
    \begin{subfigure}[b]{\linewidth}
        \centering
        \includegraphics[width=0.8\linewidth]{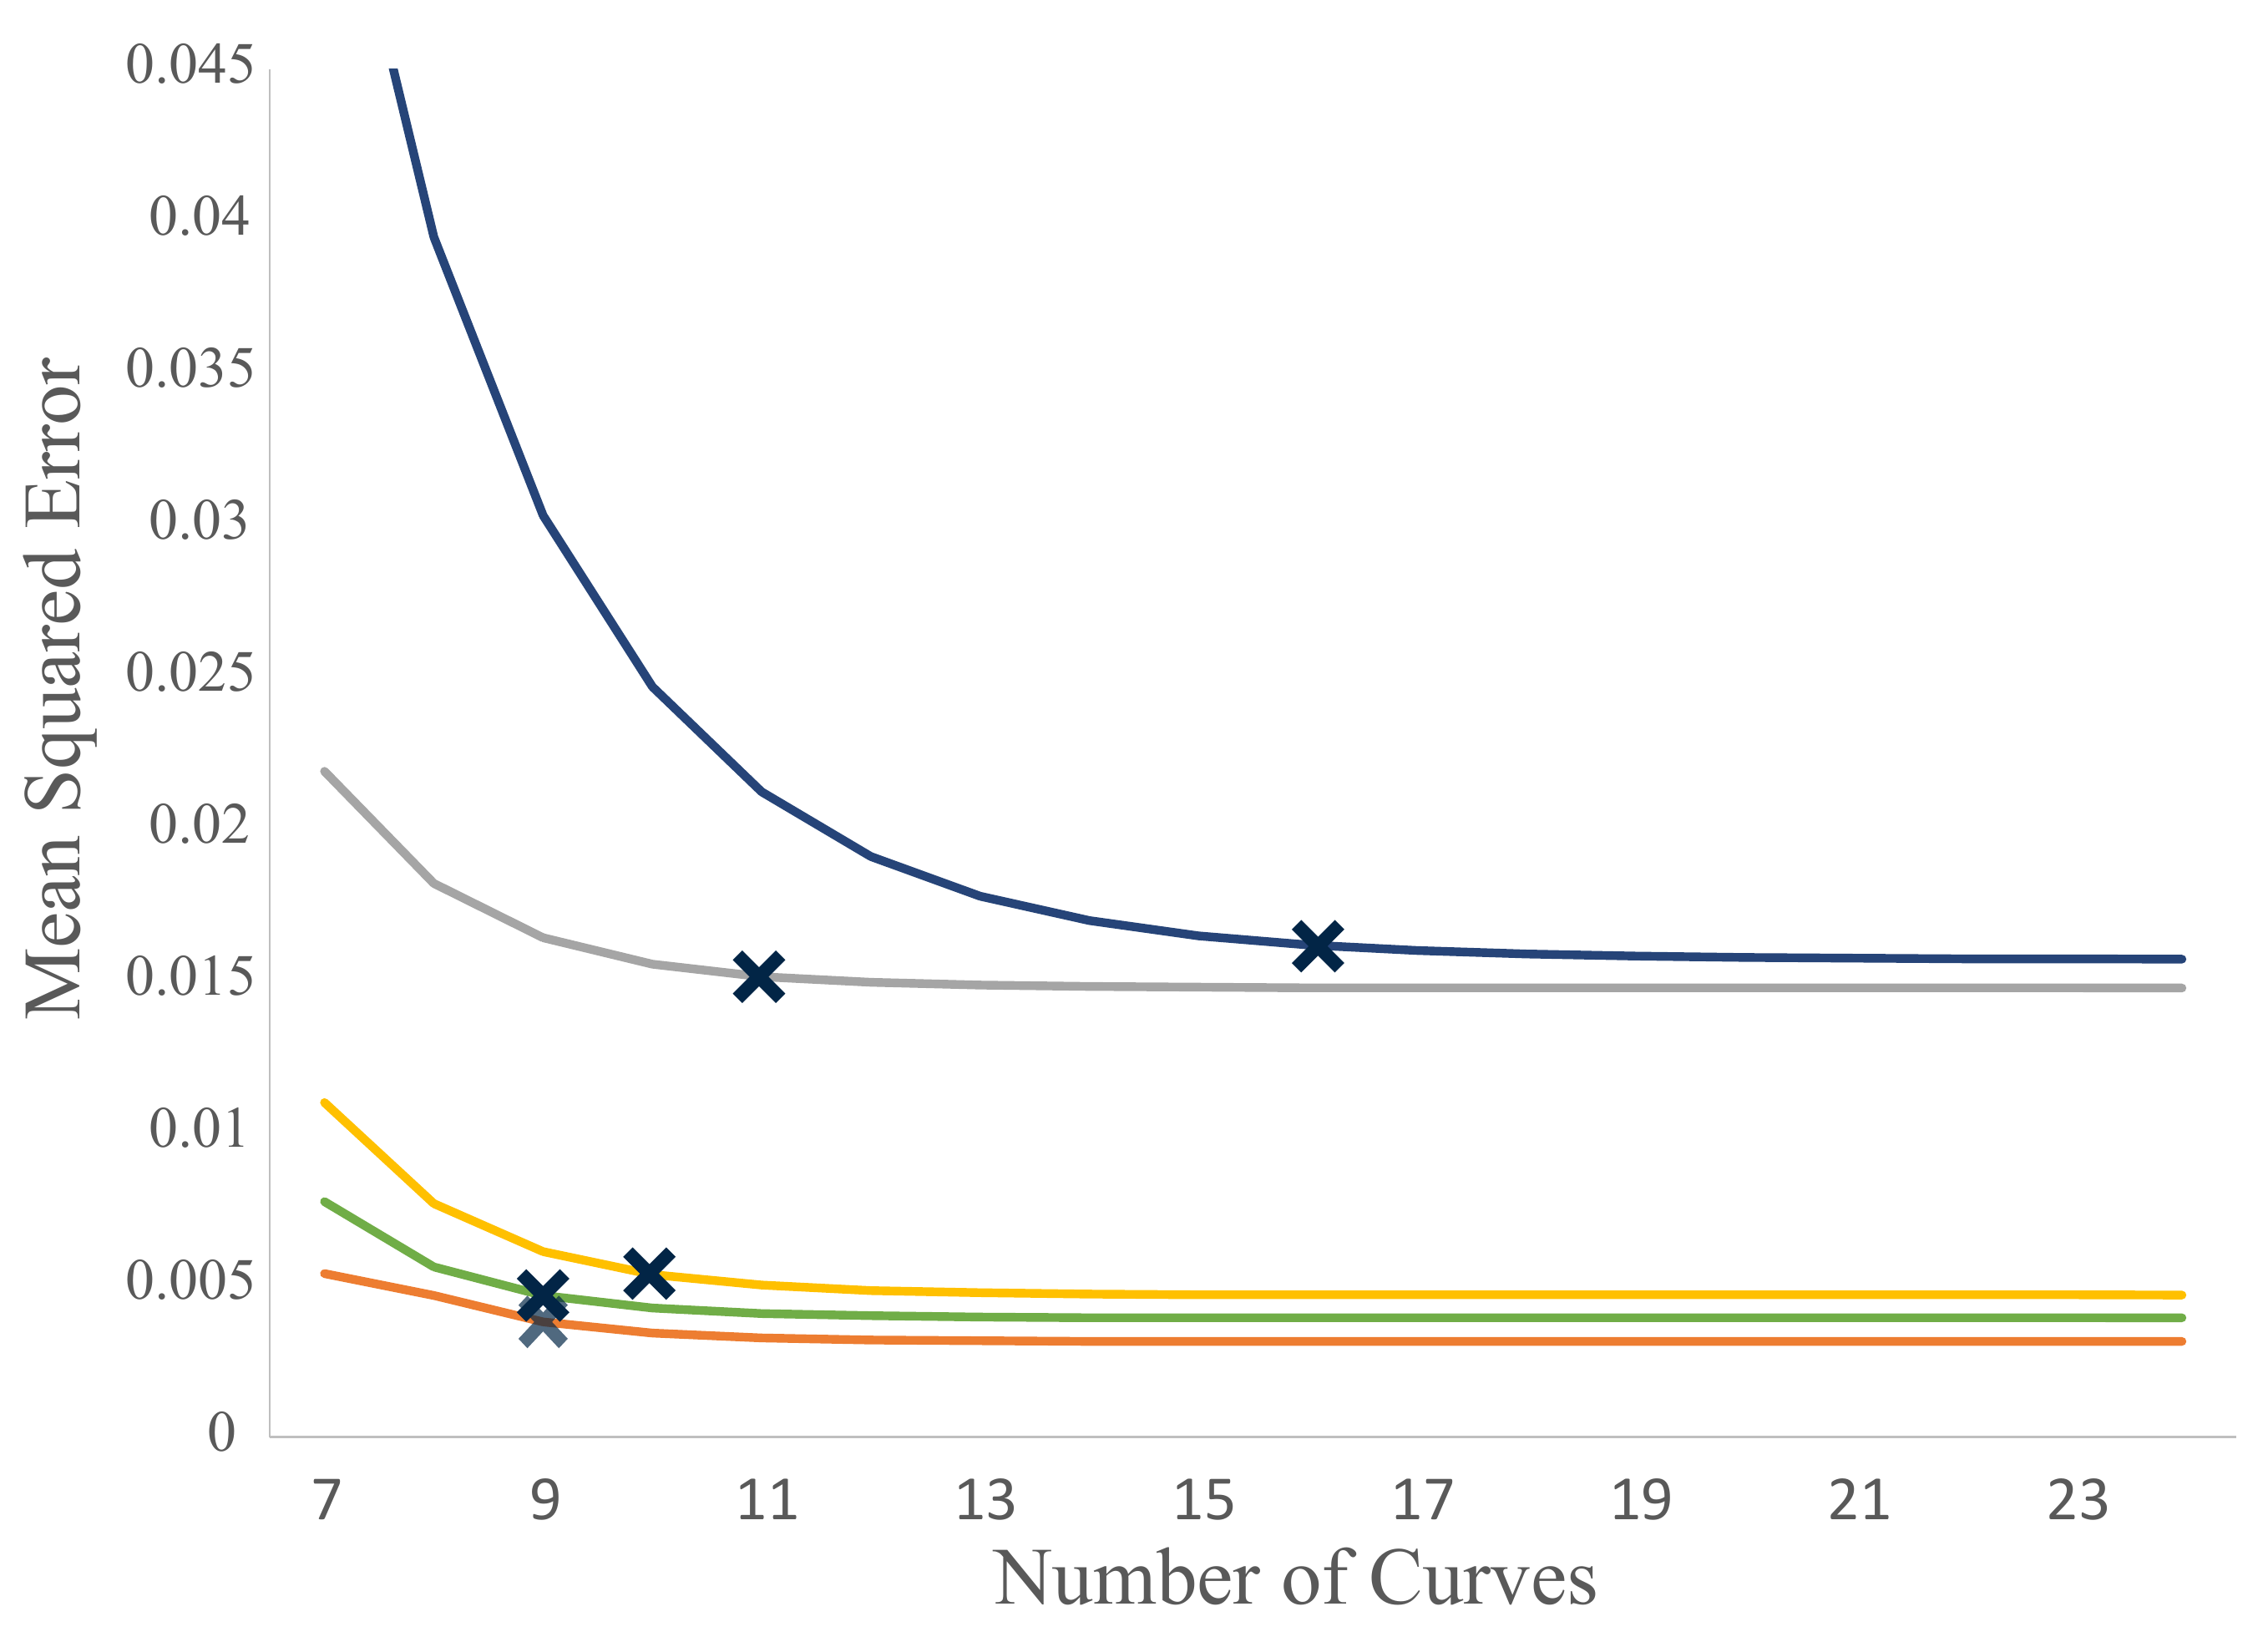}
        \caption{error vs.\ number of segments; modelled\label{fig:graph_modelled}}
    \end{subfigure}

    % \end{subfloat}
    \caption{\label{fig:sample_deform_graph_supp}
    {\bf Auxillary network output.}
    Our auxiliary network helps us choose the best sampling density on the unit circle, such that we express the generated shape with the fewest number of B\'ezier curves based on the user defined reconstruction error threshold.
    }
\end{figure}

\section{ Auxiliary Network}
In Figure \ref{fig:graph_gt},   we plot the reconstruction error vs.\ number of path segments for 5 randomly sampled instances from the \Fonts dataset, as estimated by our trained Im2Vec model.
In  Figure \ref{fig:graph_modelled}, we show a plot of the reconstruction error vs.\ the number of segments modelled by our auxiliary network. We use Equation~\eqref{eq:derived_k} to select the appropriate sampling rate for new shapes generated using our method. This enables us represent each of the generated shape in the most compact way. We mark `x' in the Figure \ref{fig:graph_modelled} for k =  0.005.

\textbf{N = number of curves} and 
\textbf{k = Rate of change of loss.}
\begin{align}
\label{eq:derived_k}
&&\text{loss}  =  c + \exp(b-a*N) \\
&&d\text{loss}/dN  =  -a  \exp(b-a*N)\\
\implies &&k >  -a   \exp(b-a*N)\\
\implies &&k/a   <  \exp(b-a*N)\\
\implies &&\log(k/a)  <  b -a*N\\
\implies &&-b + \log(k/a) <  -a*N\\
\implies&& -\log(k/a)  + b >  a*N\\
\implies &&\frac{\log(a/k)  + b}{a} >   N
\end{align}

\section{Robustness to Inconsistent Correspondence}
In Section 3.4 of the main paper, we describe a pipeline that segments the sub-components of a design or font, using off-the-shelf tools, which improves the interpretability and consistency of latent space interpolations.
In Figure~\ref{fig:inconsistent_coloring}, we show that differential compositing makes our method robust to potential inconsistencies in this automatic labelling step.
For this experiment, we specifically created training and test datasets of font character `8' where the openings are colored inconsistently.
Note that our model still manages to capture meaningful interpolations for instances that have consistent labels.
\begin{figure}
    \centering
    \includegraphics[width=\linewidth]{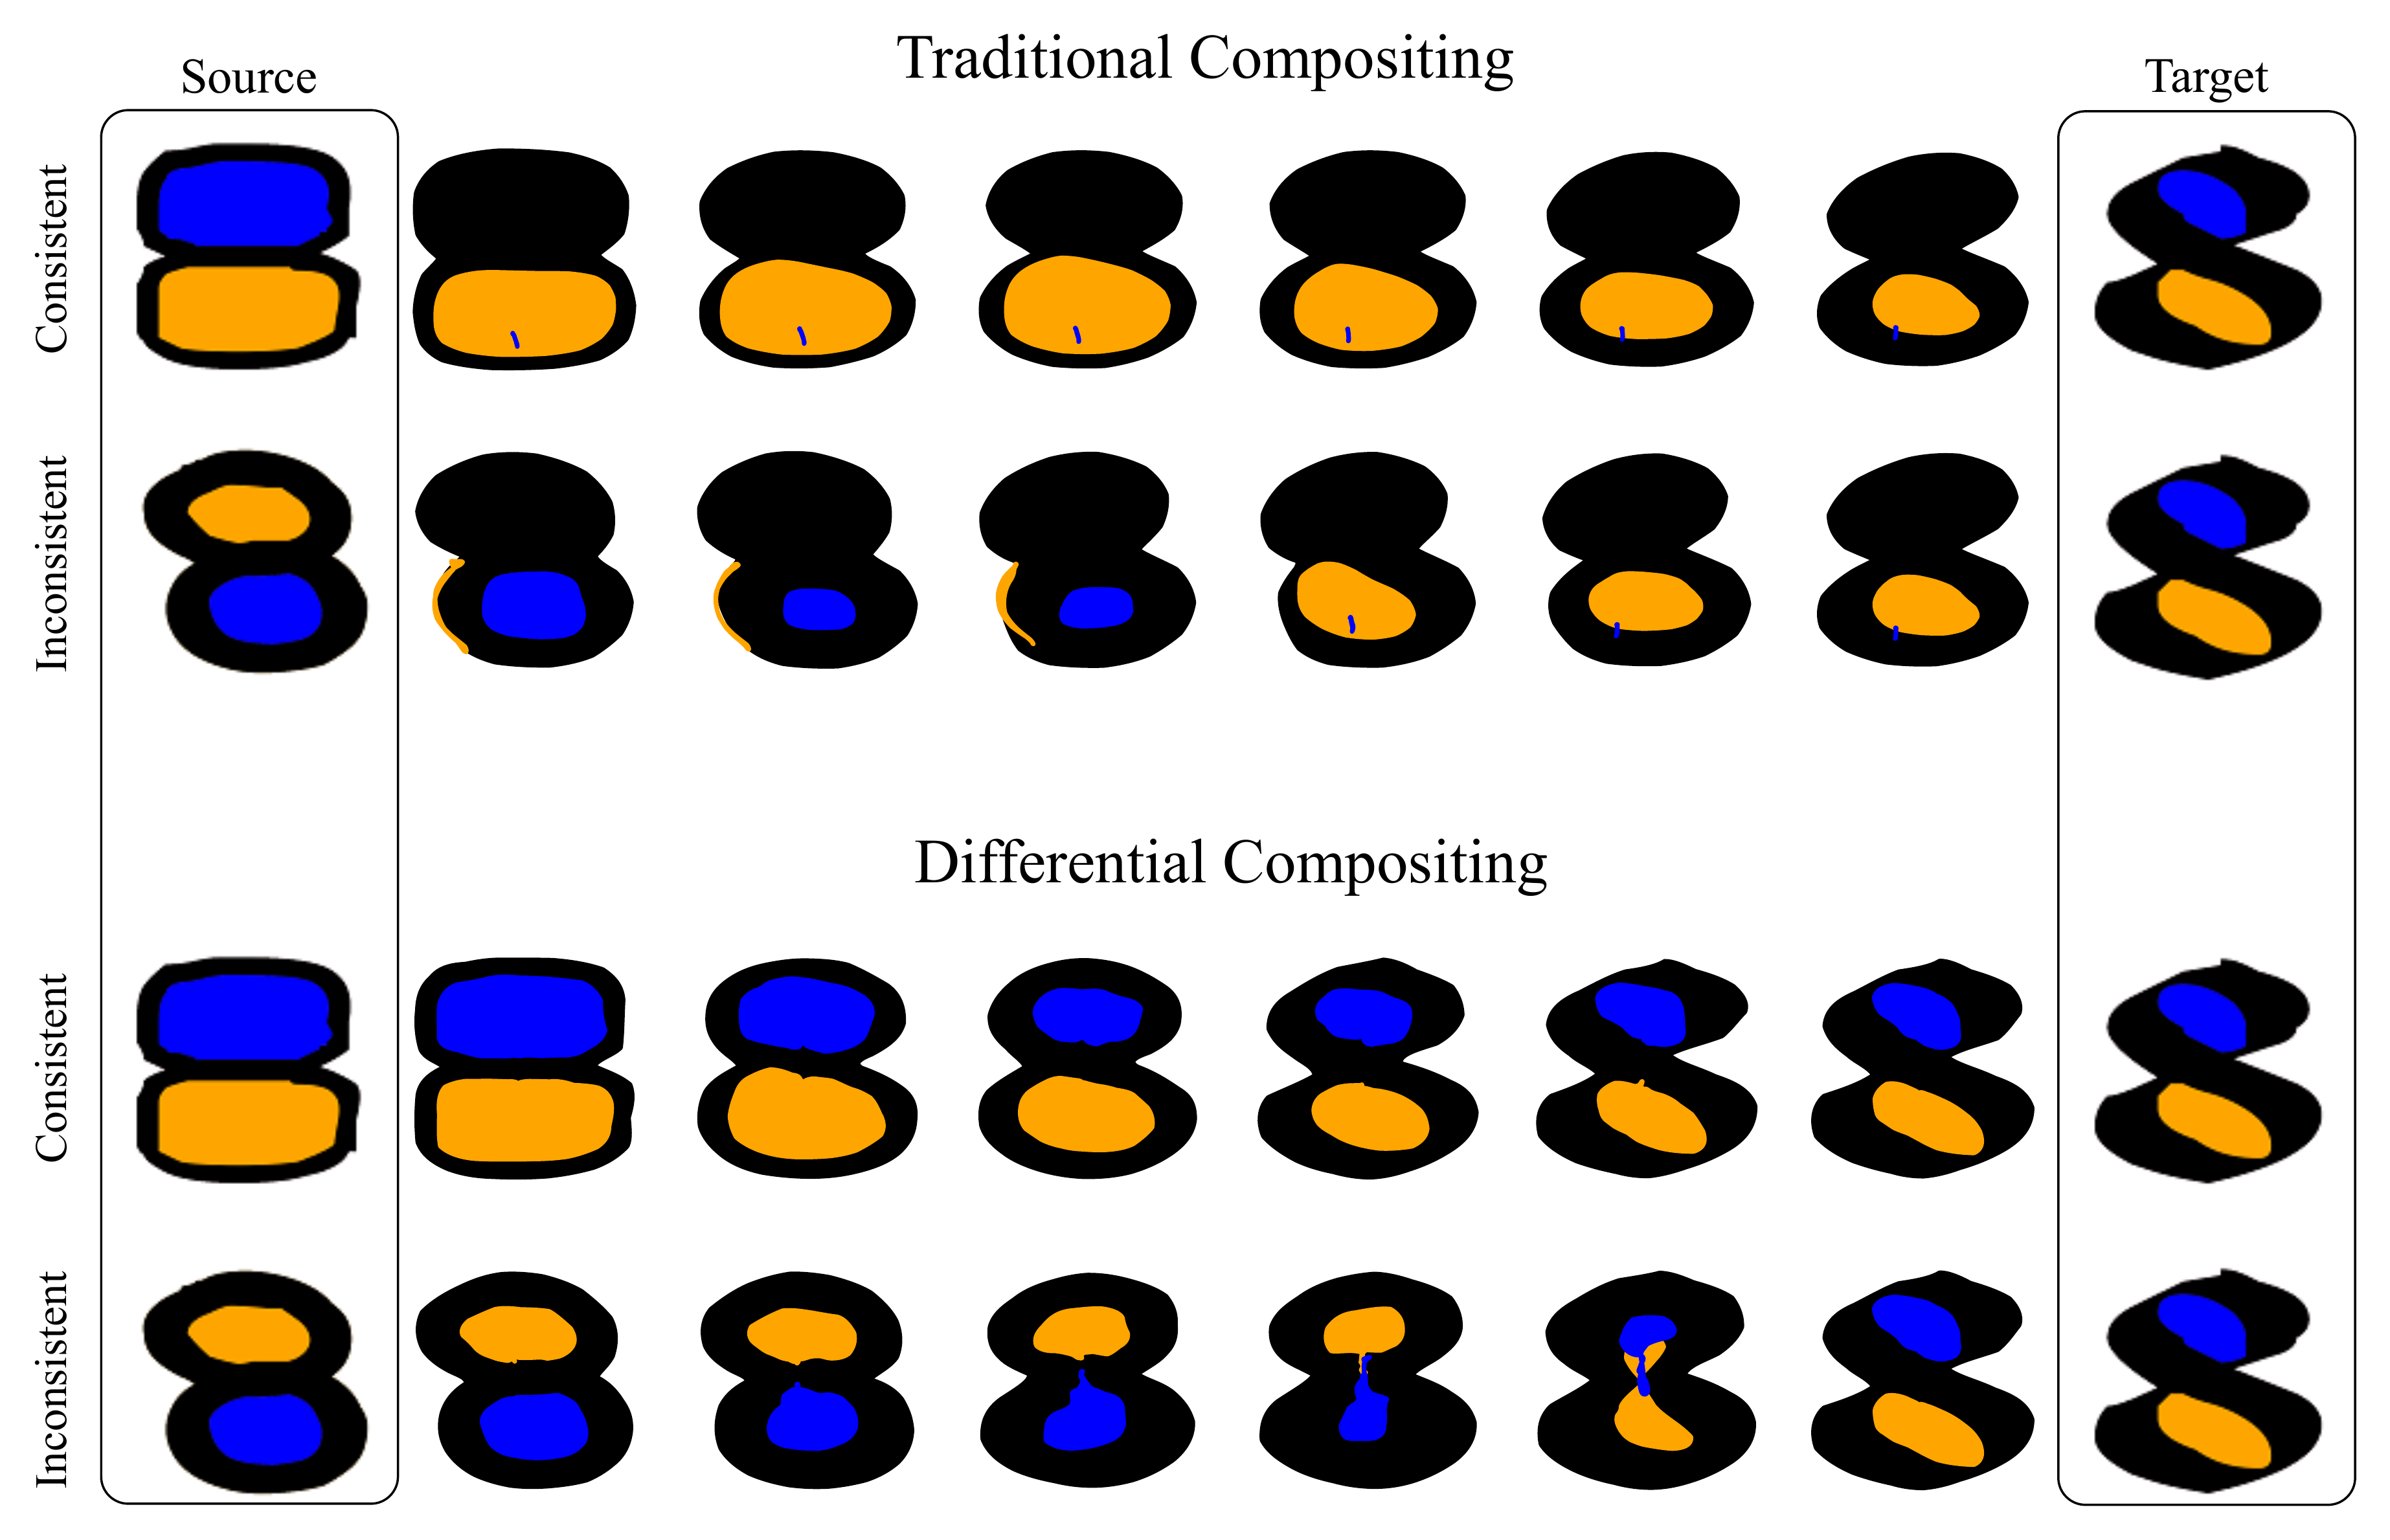}
    \caption{
        {\bf Training on inconsistent dataset.}
        We show latent space interpolations using models trained with traditional compositing versus differential  compositing. In both the scenarios, we show examples of interpolations between consistently labelled instances and inconsistently labelled instances. When trained with differential compositing, in both the scenarios our model is robust to  pre-processing inconsistencies.
    }
    \label{fig:inconsistent_coloring}
\end{figure}

\section{Code}
We also include a development version of our code in the supplemental folder to help the reader reproduce our results.
